# Supplementary material for: DoraemonGPT: Toward Understanding Dynamic Scenes with Large Language Models (Exemplified as A Video Agent)
Source: arXiv:2401.08392 source file (2025-03-06)
Supplement: Supplementary file 2 [file supp_sdm_time.tex]

\begin{table}[h]
\centering
\caption{Time Analysis of Space-Dominant Memory Construction.}
\label{tbl:supp_sdm_time}

\small
\begin{tabular}{|c|c|c|c|c|c|}
    \hline\thickhline
    \rowcolor{mygray}
Model & \makecell{ BLIP-2 \\ \cite{li2023blip}} & \makecell{ YOLO-v8 \\ \cite{yolov8}} & \makecell{ Deep OC-Sort \\ \cite{maggiolino2023deep}} & \makecell{ InternVideo \\ \cite{wang2022internvideo}} & Sum \\
    \hline\hline
Time(s) & 0.09 & 0.16 & 0.14 & 0.03 & 0.42 \\
    \hline
\end{tabular}
\end{table}

% YOLOv8~\cite{yolov8}
% Deep OC-sort~\cite{maggiolino2023deep}
% BLIP~\cite{li2022blip}/BLIP-2~\cite{li2023blip}/InstructBLIP~\cite{Dai2023InstructBLIPTG})
% InternVideo~\cite{wang2022internvideo}
% Whisper~\cite{radford2023robust}
% OCR~\cite{ocr}
