# Supplementary material for: DoraemonGPT: Toward Understanding Dynamic Scenes with Large Language Models (Exemplified as A Video Agent)
Source: arXiv:2401.08392 source file (2025-03-06)
Supplement: Supplementary file 3 [file supp_tdm_time.tex]

\begin{table}[h]
\centering
\caption{Time Analysis of Time-Dominant Memory Construction.}
\label{tbl:supp_tdm_time}

\small
\begin{tabular}{|c|c|c|c|c|}
    \hline\thickhline
    \rowcolor{mygray}
Model & OCR~\cite{ocr} & Whisper~\cite{radford2023robust} & BLIP-2~\cite{li2023blip} & Sum  \\
    \hline\hline
Time(s) & 0.02 & 0.36 & 0.09 & 0.47 \\
    \hline
\end{tabular}
\end{table}

% YOLOv8~\cite{yolov8}
% Deep OC-sort~\cite{maggiolino2023deep}
% BLIP~\cite{li2022blip}/BLIP-2~\cite{li2023blip}/InstructBLIP~\cite{Dai2023InstructBLIPTG})
% InternVideo~\cite{wang2022internvideo}
% Whisper~\cite{radford2023robust}
% OCR~\cite{ocr}
