# Supplementary material for: DoraemonGPT: Toward Understanding Dynamic Scenes with Large Language Models (Exemplified as A Video Agent)
Source: arXiv:2401.08392 source file (2025-03-06)
Supplement: Supplementary file 4 [file supp_time_token.tex]

\begin{table}[h!]
\centering
\caption{Token Efficiency (Averaged on the NExT-QA~\cite{xiao2021next} s\_val).}
\label{tbl:supp_token}

\small
\begin{tabular}{|c|c|c|c|c|c|}
    \hline\thickhline
    \rowcolor{mygray}
 Method & Prompt tokens & Node tokens & \makecell[c]{Steps \\ per Solution} & \makecell[c]{Tokens \\ per Answer} & NExT-QA Acc$_\text{A}$ \\
    \hline\hline
ViperGPT~\cite{suris2023vipergpt} & 4127 & - & - & 4127 & 45.5 \\
VideoChat~\cite{li2023videochat} & 722 & - & - & \textbf{722} & 51.8 \\
    \rowcolor{mygray1} DoraemonGPT & \textbf{617} & 34.6 & 2.3 & 1498 & \textbf{55.7} \\
    \hline
\end{tabular}
\end{table}
