# Supplementary material for: DoraemonGPT: Toward Understanding Dynamic Scenes with Large Language Models (Exemplified as A Video Agent)
Source: arXiv:2401.08392 source file (2025-03-06)
Supplement: Supplementary file 5 [file supp_tvqa.tex]

\begin{table}[h]
\centering
\small
\caption{Comparison of our DoraemonGPT with SOTAs on TVQA+~\cite{lei2020tvqa+}. $\dag$: reimplement using the officially released codes.  $*$: we filter out those failed executions (\ie, compilation error) of ViperGPT~\cite{suris2023vipergpt} and record the performance on successful executions (802/900 on \texttt{s\_val}).}
\label{tbl:supp_tvqa}

\begin{tabular}{|c|c|c|}
    \hline\thickhline
    \rowcolor{mygray}
 Method & Split & Accuracy \\
    \hline\hline
$^\dag$ViperGPT~\cite{suris2023vipergpt} & s\_val & 26.8 \\
$^{*\dag}$ViperGPT~\cite{suris2023vipergpt} & s\_val & 30.1 \\
$^\dag$VideoChat~\cite{li2023videochat} & s\_val & 34.4 \\
    \rowcolor{mygray1} DoraemonGPT & s\_val & \textbf{40.3} \\
    \hline
\end{tabular}
\end{table}
